# Supplementary material for: Anderson Metal-Insulator Transitions With Classical Magnetic Impurities
Source: arXiv:1507.03374 source file (2016-02-25)
Supplement: Supplementary file 1 [file mag-amit-supp.pdf]

# Anderson Metal-Insulator Transitions With Classical Magnetic Impurities: Supplemental material

Daniel Jung* and Stefan Kettemann†
*School of Engineering and Science, Jacobs University Bremen, 28759 Bremen, Germany*

Keith Slevin‡
*Department of Physics, Graduate School of Science, Osaka University,*
*1-1 Machikaneyama, Toyonaka, Osaka 560-0043, Japan*
(Dated: October 22, 2015)

In the supplemental materials we justify our choice of the number of Chebychev moments used within the kernel polynomial method, show some preliminary results for the large coupling behavior, discuss possible correlation effects in the local density of states, estimate the spin relaxation length and introduce the goodness of fit probability that is used to assess the quality of the fits.

## INFLUENCE OF THE PARAMETER $G$

The right choice of the parameter $G = L^d/M$ is cruicial within the kernel polynomial method (KPM), where $L$ is the linear system size of a $d$-dimensional system, and $M$ is the number of Chebychev moments used within the polynomial expansion. As Chebychev polynomials are only defined on the interval $[-1, 1]$, the energy $E$ has to rescaled so that the spectrum fits into that interval. As the spectra of the considered model are already centered around $E = 0$, we can use a linear scaling like $E = a\tilde{E}$. As rescaling factor we choose $a = 24t$.

In the center of the rescaled energy interval, the broadening of a Gaussian-shaped delta-peak (eigenvalue) within the KPM approximation is given by $\tilde{\eta} = \pi/M$ [1, 2]. So in the original energy scale, the broadening is $\eta = a\tilde{\eta}$.

There are $2L^d$ states in the system (including factor 2 because of spin), so the energy-dependent level spacing is given by $\Delta(E) = (\rho(E)\, 2L^d)^{-1}$. The value of the density of states (DOS) $\rho(E)$ at the bandcenter depends on the disorder parameters $W$ and $J$. For the sake of this estimate, we use a value for average amount of disorder, $W/t = 16.5$ and $J/t = 0$, for which we find a numerical value of $\rho(0)\, t \approx 0.056$. With this, the second argument of the fit model (see main article) is

$$\frac{\eta}{\Delta} \approx 48\pi \cdot 0.056\, G \quad . \tag{1}$$

If $\eta/\Delta$ is supposed to be around 1 (or slightly above), the value of $G$ should ideally be chosen as $G \approx 0.1$. Staying slightly above this estimate should prevent the case in which no eigenvalue is found within one kernel width. However, choosing a value of $G$ that lies far above $G = 0.1$ would mix too many states, e.g. non-critical with critical ones, within the kernel width.

As the utilized KPM algorithm performs linearly with the involved matrix dimensions $2N \times 2N$ ($N = L^d$) and the number of Chebychev moments $M$ [1], the computational effort grows inversly linear with $G$. As a tradeoff between available system sizes $N$, the obtainable value of the parameter $G$ and the resulting computation times, we have chosen $G = 1$ as a compromise for our calculations in the main article. In this way, the fit results are already very satisfying for $G = 1$, with the exception of the localization length exponent $\nu$ (see main article), and they represent a big improvement over earlier attempts, where we chose $G = 20$ (see Tab. I and Fig. 1) [3]. For $G = 20$, we were not able to obtain acceptable goodness of fit (GOF) probabilities $Q$. We recommend that future investigations (of 3D systems) should use a value of the order of $G \approx 0.1$ if possible, in order to obtain most reliable results.

## QUALITATIVE RESULTS FOR THE LARGE-COUPLING BEHAVIOR

For $G = 20$, we were able to obtain more data for large coupling strength $J$, for both Heisenberg and Ising impurities, but on the downside, we were not able to fit the data in a reasonable way to the fit model (see main article), regardless of the polynomial expansion order $n_{\mathrm{F}}$, which becomes apparent from the extremly small goodness of fit (GOF) probabilities $Q$ in Tab. I. So only qualitative conclusions can be drawn from these early results.

For Heisenberg impurities, the polar angle $\theta_i$ defining the direction of the classical magnetic moment at site $i$ is drawn uniformly from the interval $\cos\theta_i \in [-1, 1]$, while for Ising impurities, it is drawn from a binary distribution, allowing only the values $\cos\theta_i \in \{-1, 1\}$. We used 5 system sizes $L \in \{10, 20, \cdots, 50\}$ and between 6 and 12 disorder strengths $W$ for each fit, roughly adjusting their range to the expected shift of $W_{\mathrm{c}}$. The number of lattice sites $p$ where the LDOS has been sampled in each disorder realization is adjusted to the system size, $p = L^3/10$.

Fig. 1 shows that while a finite coupling strength $J$ of Ising impurities lowers the critical disorder $W_{\mathrm{c}}$, in case of Heisenberg impurities, $W_{\mathrm{c}}$ is first increased to a certain maximum value of $W_{\mathrm{c}}/t \approx 20$, before it eventually decreases as well. As explained in the main article, this

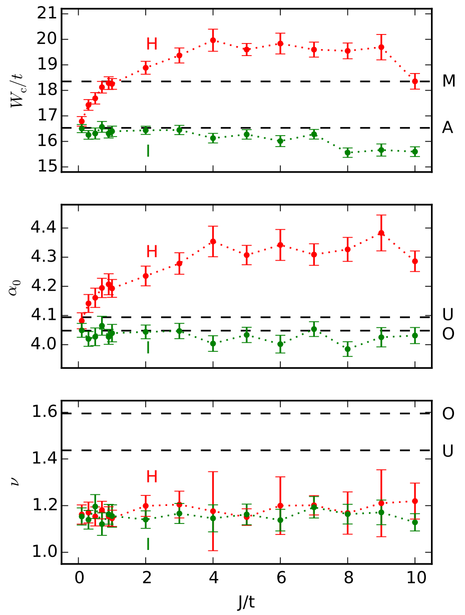


FIG. 1. (color online) Dependence of the fit parameters $W_c$, $\alpha_0$ and $\nu$ on the exchange coupling $J$ for Heisenberg (H) and Ising (I) impurities and $G = 20$. The dashed horizontals mark established values for the pure Anderson model (A, realised by our model for $J = 0$) [4], a model considering an external magnetic field (M) [5], the 3D orthogonal (O) [4, 6] and the 3D unitary (U) universality class [6]. The errorbars correspond to 95 % confidence.

boost of $W_c$ is expected, as the Heisenberg impurities change the symmetry class of the system from orthogonal to unitary. Also the parameter $\alpha_0$ is affected by the change of symmetry, while for Ising impurities, it stays at the orthogonal value.

## CORRELATION EFFECTS IN THE LDOS RAW DATA

The local density of states (LDOS) is spatially correlated. The correlation decreases with increasing distance between two points in space. In the present study (see main article), we averaged the LDOS not only over different (statistically independent) disorder realizations, but also over a fixed number of $p = 32$ lattice sites per realization, to save some computational effort when generating the realizations. The lattice sites are chosen randomly from the set of all lattice sites. Especially for small system sizes, it is not excluded that the distance between lattice sites becomes quite small. In effect, the estimated statistical error (standard error of the mean) might be too small to reflect the actual accuracy of the averaged data, as correlated states do not further increase the accuracy of the average. This can lead to fits with a reduced $\chi^2$ statistic much greater than one, and hence to a very small GOF probability $Q$ that lies outside of any acceptable range (e.g., $Q \in [0.1, 0.9]$). We recommend that future investigations should make sure that the distance between lattice sites of the same realization is large. If feasible, only one lattice site per realization should be considered, which would prevent any possibility for correlation effects.

TABLE I. Resulting fit parameters $W_c$, $\alpha_0$ and $\nu$ for the different exchange coupling strengths $J$, including their standard errors, for Heisenberg and Ising impuritires and $G = 20$. The function $\tilde{F}(x)$ has been expanded to order $n_F = 2$, so the fit model includes a total of 6 fit parameters. To assess the quality of the fit, we provide the $\chi^2$ statistic and the goodness of fit probability $Q$.

| $J/t$ | $N_D$ | $W_c/t$ | $\alpha_0$ | $\nu$ | $\chi^2$ | $Q$ |
|---|---|---|---|---|---|---|
| Anderson model | | | | | | |
| 0 | 50 | $16.19 \pm 0.10$ | $4.01 \pm 0.01$ | $1.17 \pm 0.03$ | 287.8 | $2 \cdot 10^{-37}$ |
| Heisenberg impurities | | | | | | |
| 0.1 | 40 | $16.79 \pm 0.09$ | $4.08 \pm 0.01$ | $1.16 \pm 0.02$ | 107.1 | $2 \cdot 10^{-9}$ |
| 0.3 | 40 | $17.43 \pm 0.11$ | $4.14 \pm 0.02$ | $1.17 \pm 0.02$ | 128.9 | $6 \cdot 10^{-13}$ |
| 0.5 | 60 | $17.69 \pm 0.11$ | $4.16 \pm 0.02$ | $1.15 \pm 0.02$ | 333.7 | $6 \cdot 10^{-42}$ |
| 0.7 | 50 | $18.12 \pm 0.11$ | $4.19 \pm 0.02$ | $1.18 \pm 0.02$ | 211.3 | $1 \cdot 10^{-23}$ |
| 0.9 | 50 | $18.28 \pm 0.12$ | $4.21 \pm 0.02$ | $1.15 \pm 0.02$ | 260.7 | $1 \cdot 10^{-32}$ |
| 1 | 50 | $18.25 \pm 0.11$ | $4.19 \pm 0.02$ | $1.15 \pm 0.02$ | 194.1 | $9 \cdot 10^{-21}$ |
| 2 | 50 | $18.88 \pm 0.13$ | $4.24 \pm 0.02$ | $1.20 \pm 0.02$ | 213.3 | $5 \cdot 10^{-24}$ |
| 3 | 50 | $19.37 \pm 0.15$ | $4.28 \pm 0.02$ | $1.20 \pm 0.03$ | 246.3 | $6 \cdot 10^{-30}$ |
| 4 | 30 | $19.96 \pm 0.22$ | $4.35 \pm 0.03$ | $1.18 \pm 0.08$ | 149.8 | $4 \cdot 10^{-20}$ |
| 5 | 70 | $19.60 \pm 0.12$ | $4.31 \pm 0.02$ | $1.15 \pm 0.02$ | 421.6 | $4 \cdot 10^{-54}$ |
| 6 | 30 | $19.83 \pm 0.20$ | $4.34 \pm 0.03$ | $1.20 \pm 0.06$ | 160.0 | $5 \cdot 10^{-22}$ |
| 7 | 60 | $19.60 \pm 0.15$ | $4.31 \pm 0.02$ | $1.20 \pm 0.02$ | 339.9 | $4 \cdot 10^{-43}$ |
| 8 | 30 | $19.55 \pm 0.15$ | $4.33 \pm 0.02$ | $1.17 \pm 0.05$ | 104.9 | $4 \cdot 10^{-12}$ |
| 9 | 30 | $19.69 \pm 0.25$ | $4.38 \pm 0.03$ | $1.21 \pm 0.07$ | 209.8 | $1 \cdot 10^{-31}$ |
| 10 | 40 | $18.35 \pm 0.15$ | $4.29 \pm 0.02$ | $1.22 \pm 0.04$ | 142.1 | $4 \cdot 10^{-15}$ |
| Ising impurities | | | | | | |
| 0.1 | 40 | $16.50 \pm 0.08$ | $4.05 \pm 0.01$ | $1.15 \pm 0.02$ | 96.1 | $8 \cdot 10^{-8}$ |
| 0.3 | 40 | $16.25 \pm 0.08$ | $4.02 \pm 0.01$ | $1.14 \pm 0.02$ | 111.1 | $4 \cdot 10^{-10}$ |
| 0.5 | 40 | $16.31 \pm 0.11$ | $4.03 \pm 0.02$ | $1.20 \pm 0.03$ | 151.6 | $9 \cdot 10^{-17}$ |
| 0.7 | 40 | $16.57 \pm 0.11$ | $4.06 \pm 0.02$ | $1.12 \pm 0.02$ | 184.9 | $1 \cdot 10^{-22}$ |
| 0.9 | 40 | $16.31 \pm 0.09$ | $4.03 \pm 0.01$ | $1.16 \pm 0.02$ | 114.7 | $1 \cdot 10^{-10}$ |
| 1 | 40 | $16.39 \pm 0.10$ | $4.04 \pm 0.01$ | $1.16 \pm 0.02$ | 154.4 | $3 \cdot 10^{-17}$ |
| 2 | 40 | $16.43 \pm 0.08$ | $4.04 \pm 0.01$ | $1.14 \pm 0.02$ | 99.1 | $3 \cdot 10^{-8}$ |
| 3 | 40 | $16.45 \pm 0.09$ | $4.05 \pm 0.01$ | $1.17 \pm 0.02$ | 118.7 | $3 \cdot 10^{-11}$ |
| 4 | 30 | $16.13 \pm 0.09$ | $4.00 \pm 0.01$ | $1.15 \pm 0.03$ | 73.1 | $7 \cdot 10^{-7}$ |
| 5 | 40 | $16.27 \pm 0.09$ | $4.03 \pm 0.01$ | $1.16 \pm 0.02$ | 116.5 | $6 \cdot 10^{-11}$ |
| 6 | 40 | $16.01 \pm 0.11$ | $4.00 \pm 0.02$ | $1.14 \pm 0.02$ | 172.2 | $2 \cdot 10^{-20}$ |
| 7 | 40 | $16.28 \pm 0.09$ | $4.05 \pm 0.01$ | $1.19 \pm 0.02$ | 104.9 | $4 \cdot 10^{-9}$ |
| 8 | 40 | $15.56 \pm 0.09$ | $3.98 \pm 0.01$ | $1.16 \pm 0.02$ | 113.5 | $2 \cdot 10^{-10}$ |
| 9 | 40 | $15.66 \pm 0.12$ | $4.03 \pm 0.02$ | $1.17 \pm 0.03$ | 181.7 | $4 \cdot 10^{-22}$ |
| 10 | 50 | $15.60 \pm 0.09$ | $4.03 \pm 0.01$ | $1.13 \pm 0.02$ | 209.9 | $2 \cdot 10^{-23}$ |

## THE SPIN RELAXATION LENGTH

The symmetry parameter $X_\mathrm{s} = \xi^2/L_\mathrm{s}^2$ determines the symmetry class of the system. If $X_\mathrm{s} < 1$, we are in the orthogonal symmetry class, while for $X_\mathrm{s} > 1$, we are in the unitary symmetry class. $X_\mathrm{s}$ is a function of the disorder parameter $W$ and the exchange coupling strength $J$. Our analysis builds on analytical results which rely on a scaling with $X_\mathrm{s}$. To make this scaling possible, the parameter $X_\mathrm{L} = L^2/L_\mathrm{s}^2$ must be kept to values larger than 1. So it is crucial that this condition is fulfilled for our chosen parameter combinations $(J, W, L)$.

To estimate the value of $X_\mathrm{L}$ for our numerical calculations, we consider the diffusion constant

$$D_\mathrm{e} = \frac{\langle \mathbf{v}^2 \rangle \tau}{d} \quad , \tag{2}$$

where $\langle \mathbf{v}^2 \rangle$ is the group velocity of the electrons on the Fermi surface, averaged over all angles. $\tau^{-1} = \tau_0^{-1} + \tau_\mathrm{s}^{-1}$ is the total scattering rate, with the nonmagnetic scattering rate $\tau_0^{-1} = 2\pi W^2 \rho(\varepsilon_\mathrm{F})/(6\hbar)$ and the spin scattering rate $\tau_\mathrm{s}^{-1}$ is defined by

$$\tau_\mathrm{s}^{-1} = \frac{2\pi}{\hbar} n_\mathrm{M} S^2 J^2 \rho(\varepsilon_\mathrm{F}) \quad , \tag{3}$$

where $\rho(\varepsilon_\mathrm{F})$ is the total density of states at the Fermi energy. The Fermi energy $\varepsilon_\mathrm{F}$ is taken at the band center, $\varepsilon_\mathrm{F} = D/2$. In our tight binding model, the bandwidth is $D = 12t$.

For the sake of this estimate, we use the *parabolic approximation* for the dispersion relation, although this might lead to a certain overestimation at the band center. Then, we can use the *effective mass*

$$m = \frac{1}{2t}\frac{\hbar^2}{a^2} \quad , \tag{4}$$

with the lattice spacing $a$. By using the kinetic energy

$$\varepsilon_\mathrm{F} = \frac{1}{2} m\, v_\mathrm{F}^2 \tag{5}$$

and $d = 3$ we are able to compute the average group velocity as

$$\langle \mathbf{v}^2 \rangle = v_\mathrm{F}^2 = 24t^2 \frac{a^2}{\hbar^2} \quad . \tag{6}$$

Fig. 2 illustrates how $X_\mathrm{L}$ depends on $J$ for the different system sizes. Following this rough estimate, we get $X_\mathrm{L} > 1$ for most of our systems. Only for small coupling strength, $J/t \leq 0.2$, $L_\mathrm{s}$ exceeds the smaller system sizes. In order to make sure that $X_\mathrm{L} > 1$ for all considered parameter combinations $(J, W, L)$, future investigations should consider larger systems.

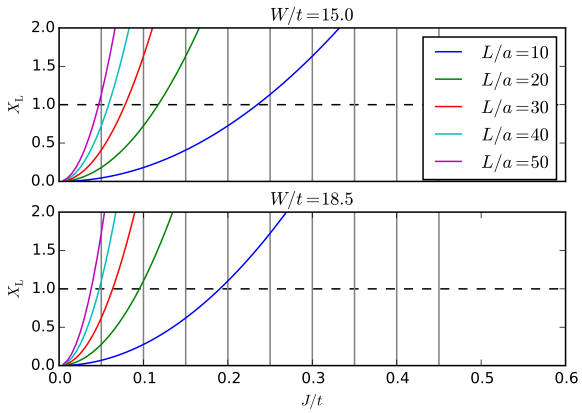


FIG. 2. (color online) Dependence of the parameter $X_\mathrm{L}$ on the exchange coupling strength $J$ for our considered linear system sizes $L$ and the smallest and largest considered disorder parameters $W$. The vertical gray lines mark our considered $J$ values.

## THE GOODNESS OF FIT PROBABILITY

To assess the quality of the fits, we compute the *goodness of fit probability* (GOF) [7]

$$Q = \int_{\chi^2}^{\infty} p(x, k)\, \mathrm{d}x \quad , \tag{7}$$

where

$$p(x, k) = \frac{x^{(k-2)/2} e^{-x/2}}{2^{k/2}\Gamma(k/2)} \tag{8}$$

is the *chi-squared distribution* [7] and $k = N_\mathrm{D} - N_\mathrm{P}$ is the number of *degrees of freedom* (DOF). $N_\mathrm{D}$ is the number of data points and $N_\mathrm{P}$ the number of fit parameters in the fit model.

* d.jung@jacobs-university.de
† s.kettemann@jacobs-university.de
‡ slevin@phys.sci.osaka-u.ac.jp

[1] A. Weiße, G. Wellein, A. Alvermann, and H. Fehske, Rev. Mod. Phys. **78**, 275 (2006).
[2] G. Schubert, and H. Fehske, in *Quantum and Semi-classical Percolation and Breakdown in Disordered Solids*, edited by Bikas K. Chakrabarti, Kamal K. Bardhan, and Asok K. Sen, Lecture Notes in Physics Vol. 762 (Springer, Berlin, Heidelberg, 2009).
[3] D. Jung, and S. Kettemann, AIP Conf. Proc. **1610**, 77 (2014).
[4] A. Rodriguez, L. J. Vasquez, K. Slevin, and R. Römer, Phys. Rev. B **84**, 134209 (2011).
[5] T. Dröse, M. Batsch, I. Zharekeshev, and B. Kramer, Phys. Rev. B **57**, 37 (1998).

[6] L. Ujfalusi, and I. Varga, Phys. Rev. B **91**, 184206 (2015).

[7] P. Bevington, and D. Robinson, *Data Reduction and Error Analysis for the Physical Sciences*, McGraw-Hill Education, Boston (2002).
